# Supplementary material for: Decentralized State Estimation In A Dimension-Reduced Linear Regression
Source: arXiv:2210.06947 source file (2023-12-11)
Supplement: Supplementary file 1 [file appendix.tex]

%\newpage

\appendices

\section{A Mean Squared Error Optimal Fusion Method} \label{app:optimal-fusion-rule}

%An \abbrMSE optimal method is derived for the fusion of two correlated estimates. 

Assume that
\begin{align*}
	y_1 &= x + v_1, & R_1 &= \cov(v_1), &
	y_2 &= H_2x + v_2, & R_2 &= \cov(v_2),
\end{align*}	
with $R_{12}=\cov(v_1,v_2)$. Let $\yM=\M y_2$ and $\RM=\M R_2\Mt$, where $\M\in\realsmnb$, $m\leq\nb$ and $\rank(\M)=m$, such that $R_{1\M}=\cov(v_1,\M v_2)=R_{12}\Mt$. The goal is to compute an estimate $\xhat=K\col(y_1,\yM)$, with $KH=I$ and $H=\col(I,\M H_2)$, that minimizes trace of 
\begin{equation*}
	P = K\BBM R_1&R_{1\M}\\ R_{\M1}&\RM\EBM K\trnsp.
\end{equation*}
Let $K=\BBM K_1&\KM\EBM$ such that $KH=I\implies K_1 = I-\KM\M H_2$. Let $R\succeq0$ and $S=H_2R_1H_2\trnsp+R_2-H_2R_{12}-R_{21}H_2\trnsp\succeq0$, but assume $\M$ is such that $\M S\Mt\succ0$. Since $K=\BBM I-\KM\M H_2&\KM\EBM$
\begin{align*} 
	P
	&= R_1 - R_1H_2\trnsp\Mt \KM\trnsp - \KM\M H_2 R_1 + \KM\M H_2 R_1H_2\trnsp\Mt \KM\trnsp \\ 
	&\quad + \KM R_{\M1} - \KM R_{\M1}H_2\trnsp\Mt\KM\trnsp + R_{1\M}\KM\trnsp \\
	&\quad - \KM\M H_2R_{1\M}\KM\trnsp + \KM\RM\KM\trnsp \\
	&=R_1 - \KM(\M H_2 R_1-R_{\M1}) - (R_1H_2\trnsp\Mt-R_{1\M})\KM\trnsp \\ 
	&\quad + \KM(\M H_2 R_1H_2\trnsp\Mt + \RM - \M H_2 R_{1\M})\KM\trnsp - R_{\M1}H_2\trnsp\Mt \\
	&=R_1 - \KM A - A\trnsp \KM\trnsp + \KM B\KM\trnsp,
\end{align*}
where
\begin{align*}
	A &= \M H_2 R_1-R_{\M1} = \M\left(H_2R_1-R_{21}\right), \\
	B &= \M H_2 R_1H_2\trnsp\Mt + \RM - \M H_2 R_{1\M} - R_{\M1}H_2\Mt \\
	&= \M\left(H_2R_1H_2\trnsp + R_2 - H_2R_{12} - R_{21}H_2\trnsp\right)\Mt = \M S\Mt.
\end{align*}	
Completing the square yields
\begin{align*}
	P = R_1 - A\trnsp B\inv A + (\KM-A\trnsp B\inv)B(\KM\trnsp-B\inv A),
\end{align*}
which is minimized when $\KM=A\trnsp B\inv$. An \abbrMSE optimal estimate is given by 
\begin{align*}
	\xhat &= K_1y_1 + \KM\yM, &
	P &= R_1 - \KM\M S\Mt \KM\trnsp, \\
	K_1 &= I-\KM\M H_2, &
	\KM &= (R_1H_2\trnsp-R_{12})\Mt(\M S\Mt)\inv, 
\end{align*}	
where $S = H_2R_1H_2\trnsp+R_2-H_2R_{12}-R_{21}H_2\trnsp$.
